# Supplementary material for: Simple Round Compression for Parallel Vertex Cover
Source: arXiv:1709.04599 source file (2017-09-14)
Supplement: Supplementary file 1 [file appendix-lower.tex]

\section{Proof of Lemma~\ref{lem:matching-dist-large}}\label{app:large-induced-matching}

Consider the edges of $\Eab$ assigned to the graph $\Gii$. It is easy to see that by the choice of $\Eab$ and further partitioning the edges between the $k$ players, 
the graph $\Gii$ on the set of edges $\Eab^{(i)}$ forms a random bipartite graph. Hence, proving Lemma~\ref{lem:matching-dist-large} reduces to proving the following property of 
random bipartite graphs.

Let ${\cal G}(n,n,1/n)$ denote the family of random bipartite graphs where each side of the bipartition contains $n$ vertices, and each edge is present w.p. $1/n$. 
We will show that if we sample a random graph $G \in {\cal G}(n,n,1/n)$, then w.p. at least $1 - 1/n^2$, it contains an {\em induced matching} of size $\Omega(n)$. We emphasize here that the notion of induced matching is with respect 
to the entire graph and not only with respect to the vertices included in the induced matching.

Our proof will use the following pair of elementary propositions.

\begin{proposition}
\label{prop:random1}
Suppose we assign $N$ balls uniformly at random to $M > N$ bins. Let $B$ be an arbitrary fixed subset of bins. Then with probability at least $1 - \frac{1}{N^3}$, there are at least $\left( \frac{|B|}{M} \right) \cdot \frac{N}{e} - o(N)$ bins in $B$ that contain exactly one ball, assuming $N$ is sufficiently large. 
\end{proposition}
\begin{proof}
We arbitrarily number the balls $1$ through $N$ and the bins $1$ through $M$. W.l.o.g. assume that the bins in $B$ are numbered $1$ through $|B|$.
For $1 \le i \le |B|$, let $Z_i$ be the $0/1$ random variable that indicates whether or not bin $i \in B$ receives exactly one ball, and furthermore, let $Z = \sum_{i=1}^{|B|} Z_i$. Then

$${\rm Pr}[Z_i = 1] = {N \choose 1}\cdot \left( \frac{1}{M} \right)  \cdot \left(1 - \frac{1}{M}\right)^{N-1} \ge \frac{N}{M}\cdot\left( \frac{1}{e} - o(1) \right).$$

Hence $E[Z] \ge \left( \frac{|B|}{M} \right) \cdot \frac{N}{e} - o(N)$. We now wish to argue that the value of $Z$ is concentrated around its expectation. However, we can not directly invoke the standard Chernoff bound since the variables $Z_i$'s are not independent. We will instead utilize the more general version stated in Proposition~\ref{prop:bounded-differences}.

Let $X_{j} \in [1..M]$ denote the index of the bin in which the $j_{th}$ ball lands. Given the variables $X_1, X_2, ..., X_N$, we can define the function $f(X_1, X_2, ...., X_N)$ to be the number of bins in $B$ that receive exactly one ball. Note that $f$ is completely determined by the variables $X_1, X_2, ..., X_N$ and that $E[f] = E[Z] \ge \left( \frac{|B|}{M} \right) \cdot \frac{N}{e} - o(N)$. It is easy to see that the function $f$ satisfies the Lipschitz property with $d=2$ since changing the assignment of any single ball, can reduce or increase the number of bins in $B$ with exactly one ball by at most $2$. We can thus invoke Proposition~\ref{prop:bounded-differences} with $t = 4\sqrt{N \ln N}$, completing the proof.
\end{proof}

\begin{proposition}
\label{prop:random2}
For sufficiently large $n$, with probability at least $1 - 1/n^3$, a graph $G(L \cup R, E)$ drawn from ${\cal G}(n,n,1/n)$ satisfies the following properties:
\begin{itemize}
\item[(a)] The set $S \subseteq L$ of all vertices in $L$ with degree exactly one in $G$ has size $n/e \pm o(n)$. %whose vertices have degree exactly one in $G$.
\item[(b)] The set $T \subseteq R$ of vertices defined as all vertices in $R$ with no edges to $L \setminus S$ has size at least $n/e - o(n)$.
\end{itemize}
\end{proposition}
\begin{proof}
To see property (a), let us define $0/1$ random variables $X_1, X_2, ..., X_n$ where $X_i = 1$ iff vertex $i \in L$ has degree exactly one in $G$. Then ${\rm Pr}[X_i=1] = (1-\frac{1}{n})^{n-1} = 1/e - o(1)$ for sufficiently large $n$. Thus $E[\sum_{i=1}^{n} X_i] = n/e - o(n)$, and using Chernoff bound (Proposition~\ref{prop:chernoff} with $t = 4\sqrt{n \ln n}$) implies that with probability at least $1 - 2/n^4$, there is a set $S \subseteq L$ of size $n/e \pm o(n)$ whose vertices have degree exactly one in $G$.

To see property (b), fix a set $S$ of degree $1$ vertices in $L$. Let us define $0/1$ random variables $Y_1, Y_2, ..., Y_n$ where $Y_i = 1$ iff vertex $i \in R$ receives no edges from vertices in $L \setminus S$. 
Then ${\rm Pr}[Y_i=1] = (1-\frac{1}{n})^{|L \setminus S|} \ge 1/e - o(1)$ for sufficiently large $n$. Thus $E[\sum_{i=1}^{n} Y_i] \ge n/e - o(n)$, and using Chernoff bound (Proposition~\ref{prop:chernoff} with $t = 4\sqrt{n \ln n}$) implies that with probability at least $1 - 2/n^4$, there is a set $T \subseteq R$ of size at least $n/e - o(n)$ whose vertices 
do not have any edges to $L \setminus S$.

Thus both properties (a) and (b) hold with probability at least $1 - 1/n^3$, as desired.
\end{proof}

\begin{lemma}\label{lem:random-graph}
Let $G(L \cup R, E)$ be drawn from ${\cal G}(n,n,1/n)$. Then for sufficiently large $n$, with probability at least $1 - 1/n^2$, $G$ contains an {\em induced matching} of size $n/e^3 -o(n)$.
\end{lemma}
\begin{proof}
By Proposition~\ref{prop:random2}, we know with probability at least $1 - 1/n^3$, the graph $G(L \cup R, E)$ satisfies properties (a) and (b). We will assume from here on that this event, denoted by ${\cal E}$, has occurred. We first 
observe that conditioned on the event ${\cal E}$, and for any choice of sets $S$ and $T$ as defined in Proposition~\ref{prop:random2} as well as edges from the set $L \setminus S$ to $R \setminus T$, sampling a graph $G$ from $
{\cal G}(n,n,1/n)$ is equivalent to assigning each vertex in $S$ a uniformly at random neighbor in $R$. 

Now invoking Proposition~\ref{prop:random1}, with $N = |S|$, $B = T$, we know that with 
probability at least $1 - O(1/n^3)$, there is a set $T' \subseteq T$ of size at least  

$$\frac{|T|}{n} \cdot \frac{|S|}{e} - o(|S|) = \left( \frac{1}{e} - o(1) \right) \cdot \left( \frac{n/e - o(n)}{e} \right) - o(n) \ge \frac{n}{e^3} - o(n)$$

such that each vertex in $T'$ receives exactly one ball from $S$ (i.e. receives exactly one edge from the vertices in $S$).
Let $S' \subseteq S$ be the set of vertices that ``supply a ball'' (i.e. an edge) to vertices in $T'$. Since by definition the vertices in $T$ receive edges only from $S$, and since all vertices in $S$ have degree exactly one, the set $S' \cup 
T'$ of vertices induces a matching of size at least $n/e^3 - o(n)$ in $G$, as asserted in the lemma.
\end{proof}

The lower bound in Lemma~\ref{lem:matching-dist-large} now follows from Lemma~\ref{lem:random-graph} for the family of bipartite graphs with $n/\alpha$ vertices on each side. 
The upper bound is a simple application of Chernoff bound on the number of edges from $\Ebab$ that are assigned to $\Gii$.
