# Supplementary material for: Simple Round Compression for Parallel Vertex Cover
Source: arXiv:1709.04599 source file (2017-09-14)
Supplement: Supplementary file 2 [file appendix-concentration.tex]

\section{Useful Concentration of Measure Inequalities}\label{app:concentration}

We use the following standard version of Chernoff bound (see, e.g.,~\cite{ConcentrationBook}) throughout. 

\begin{proposition}[Chernoff bound]\label{prop:chernoff}
	Let $X_1,\ldots,X_n$ be independent random variables taking values in $[0,1]$ and let $X:= \sum_{i=1}^{n} X_i$. Then, 
	\[ \Pr\paren{\card{X - \Ex\bracket{X}} > t} \leq 2 \cdot \exp\paren{-\frac{2t^2}{n}} \]
\end{proposition}

We also need the {method of bounded differences} in our proofs. A function $f(x_1,\ldots,x_n)$ satisfies the \emph{Lipschitz property} with constant $d$, iff 
for all $i \in [n]$, $\card{f(a) - f(a')} \leq d$, whenever $a$ and $a'$ differ only in the $i$-th coordinate. 

\begin{proposition}[Method of bounded differences] \label{prop:bounded-differences}
	If $f$ satisfies the Lipschitz property with constant $d$ and $X_1,\ldots,X_n$ are independent random variables, then, 
	\[ \Pr\paren{\card{f(X) - \Ex\bracket{f(X)}} > t} \leq 2 \cdot \exp\paren{-\frac{2t^2}{n\cdot d^2}} \]
\end{proposition}

A proof of this proposition can be found in~\cite{ConcentrationBook} (see Section 5).
